# Supplementary material for: PMC-CLIP: Contrastive Language-Image Pre-training using Biomedical Documents
Source: arXiv:2303.07240 source file (2023-03-13)
Supplement: Supplementary file 1 [file 07-Appendix.tex]

\section{Appendix}

% 3.6 会议TODO
% 1. Teaser用星状图，和不同数据集对比，同时展示数量和diversity
% 2.（MICCAI后）别人用了ROCO的实验结果里，我们也用PMC-OA + ROCO
% 3. 说我们的VQA和M3AE完全一样的framework，只是比较我们的backbone，也就是Pretrained Model
% 5. 在Figure1下面画进度条，把箭头省略了，把train CLIP和Finetune这一步放进去
% 7. Figure2用树状结构

In MICCAI version:
\begin{enumerate}
    \item VQA not SOTA
    \item Denoised not up-to-date
\end{enumerate}

\noindent In Next version:
\begin{enumerate}
    \item A ablation table on denoised dataset.
    \item Enlarge the collection source (inline reference, patient report).
    \item Have we exhausted the PMC(8M V.S. 2.5M)?
    \item Keyword filtering too limited.
    \item Improve performance of figure separation, subfigure-subcap alignment.
\end{enumerate}

This is appendix.

% medmnist 的所有子集
% 
% MedMNIST 的所有 subset 结果
% 
\begin{table*}[htpb]
    \centering
    \setlength{\tabcolsep}{6pt} % Default value: 6pt
    \caption{Full results on MedMNIST. Only 3/12 are shown in main text}
    \begin{tabular}{l|cc|cc|cc}
    \toprule
        % Modality & Chest X-Ray & Ultrasound	& Dermatoscope \\
        Dataset & \multicolumn{2}{c|}{PneumoniaMNIST} & \multicolumn{2}{c|}{BreastMNIST} & \multicolumn{2}{c}{DermaMNIST} \\
        Method & AUC$\uparrow$ & ACC$\uparrow$ & AUC$\uparrow$ & ACC$\uparrow$ & AUC$\uparrow$ & ACC$\uparrow$ \\
        \toprule
        ResNet50 & 96.20 & 88.40 & \cellcolor{lightergray}91.90 & 86.60 & 91.20 & 73.10 \\
        % Benchmark & \textbf{99.10} & 94.60 & 91.90 & 86.30 & 92.00 & 76.80 \\
        DWT-CV \cite{cheng2022dwt} & 95.69 & 88.67 & 89.77 & 85.68 & 91.67 & 74.75 \\ 
        SADAE \cite{ge2022self} & \cellcolor{lightergray}98.30 & \cellcolor{lightergray}91.80 & 91.50 & \cellcolor{lightergray}87.80 & \cellcolor{lightergray}92.70 & \cellcolor{lightergray}75.90 \\
        \midrule
        % PMC OA(LP) & 93.35 & 85.50 & 88.41 & 79.49 & 90.81 & 71.97 \\
        BioMed-CLIP & \cellcolor{lightgray} 99.02 & \cellcolor{lightgray}95.35 & \cellcolor{lightgray}94.56 & \cellcolor{lightgray}91.35 & \cellcolor{lightgray}93.41 & \cellcolor{lightgray}79.80 \\
     \bottomrule
    \end{tabular}
    \label{tab:MedMNIST_Appendix}
\end{table*}
